# Supplementary material for: EEC: Learning to Encode and Regenerate Images for Continual Learning
Source: arXiv:2101.04904 source file (2021-05-02)
Supplement: Supplementary file 1 [file reconstructions.tex]

\section{Reconstructed Images}
\label{sec:appendix_reconstructions}
A representative sample of reconstructed images by EEC for MNIST, SVHN and CIFAR-10 datasets after 10 tasks and ImageNet-50 dataset after 5 tasks.

\subsection{MNIST}
\begin{figure}[H]
\centering
\includegraphics[scale=0.7]{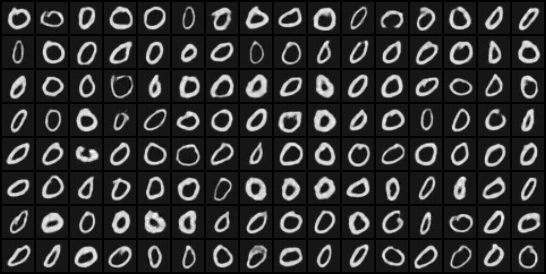}
\label{fig:mnist_0}
\end{figure}

\begin{figure}[H]
\centering
\includegraphics[scale=0.7]{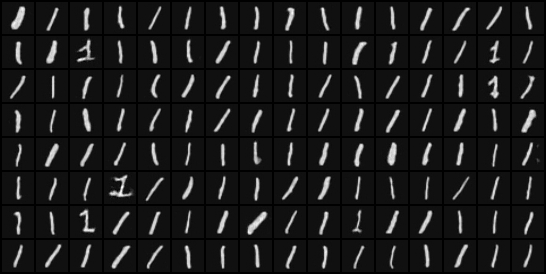}
\label{fig:mnist_1}
\end{figure}

\begin{figure}[H]
\centering
\includegraphics[scale=0.7]{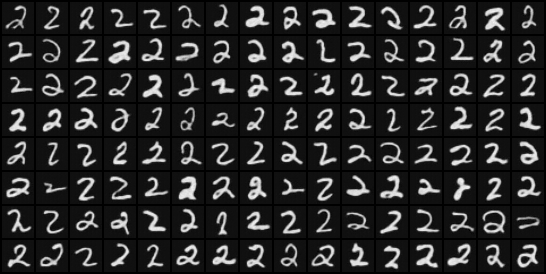}
\label{fig:mnist_2}
\end{figure}

\begin{figure}[H]
\centering
\includegraphics[scale=0.7]{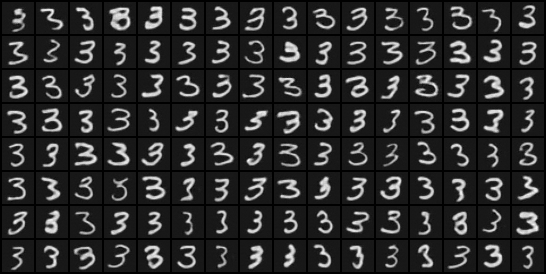}
\label{fig:mnist_3}
\end{figure}

\begin{figure}[H]
\centering
\includegraphics[scale=0.7]{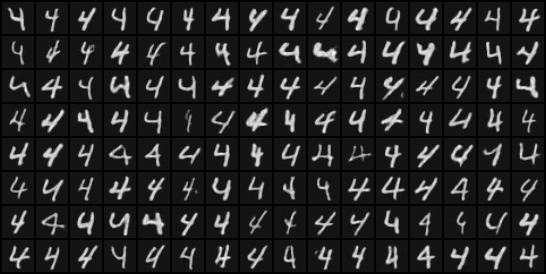}
\label{fig:mnist_4}
\end{figure}

\begin{figure}[H]
\centering
\includegraphics[scale=0.7]{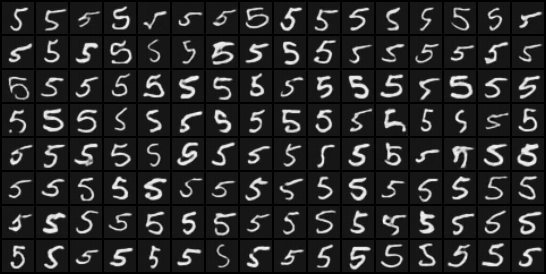}
\label{fig:mnist_5}
\end{figure}

\subsection{SVHN}
\begin{figure}[H]
\centering
\includegraphics[scale=0.7]{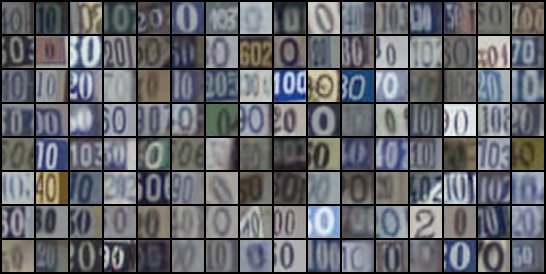}
%\caption{\small Images reconstructed by EEC for SVHN after 10 tasks}
\label{fig:svhn_0}
\end{figure}
\begin{figure}[H]
\centering
\includegraphics[scale=0.7]{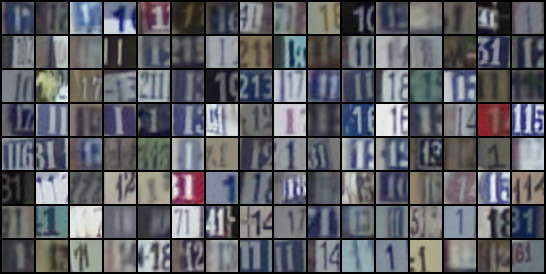}
\label{fig:svhn_1}
\end{figure}

\begin{figure}[H]
\centering
\includegraphics[scale=0.7]{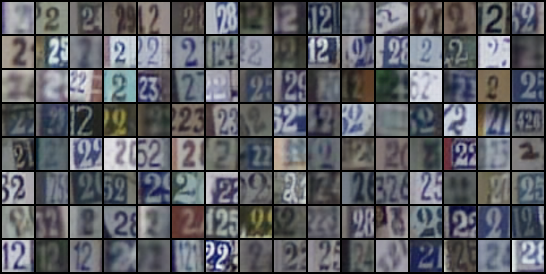}
\label{fig:svhn_2}
\end{figure}

\begin{figure}[H]
\centering
\includegraphics[scale=0.7]{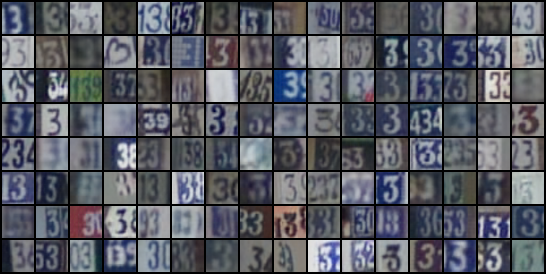}
\label{fig:svhn_3}
\end{figure}

\begin{figure}[H]
\centering
\includegraphics[scale=0.7]{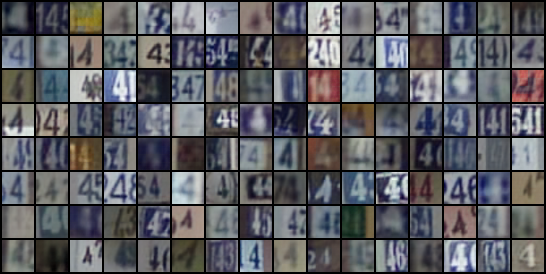}
\label{fig:svhn_4}
\end{figure}

\begin{figure}[H]
\centering
\includegraphics[scale=0.7]{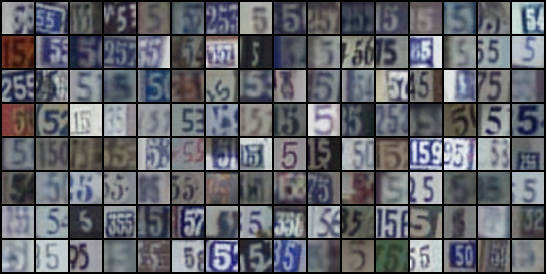}
\label{fig:svhn_5}
\end{figure}

\subsection{CIFAR-10}
\begin{figure}[H]
\centering
\includegraphics[scale=0.7]{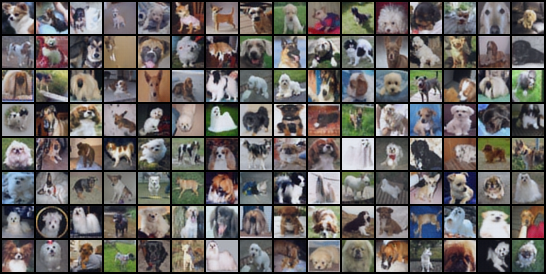}
%\caption{\small Images reconstructed by EEC for CIFAR10 after 10 tasks}
\label{fig:cifar_0}
\end{figure}
\begin{figure}[H]
\centering
\includegraphics[scale=0.7]{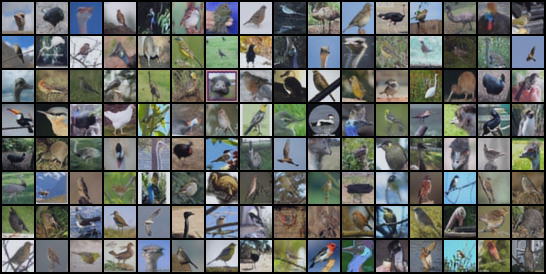}
\label{fig:cifar_1}
\end{figure}
\begin{figure}[H]
\centering
\includegraphics[scale=0.7]{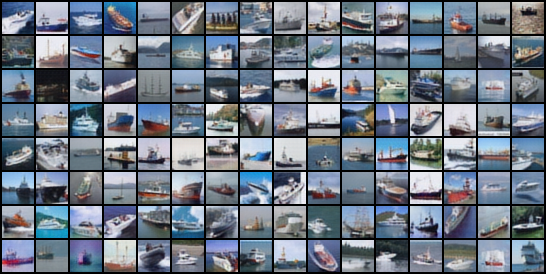}
\label{fig:cifar_2}
\end{figure}
\begin{figure}[H]
\centering
\includegraphics[scale=0.7]{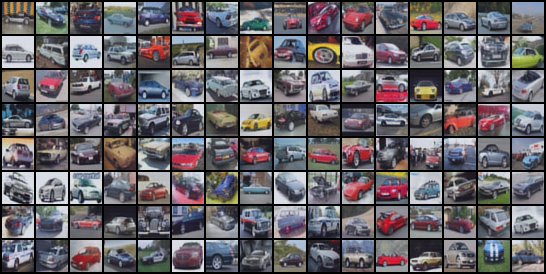}
\label{fig:cifar_3}
\end{figure}

\begin{figure}[H]
\centering
\includegraphics[scale=0.7]{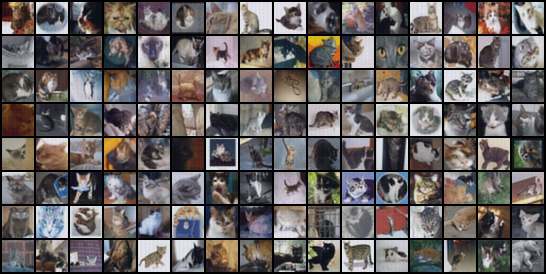}
%\caption{\small Images reconstructed by EEC for CIFAR10 after 10 tasks}
\label{fig:cifar_4}
\end{figure}

\begin{figure}[H]
\centering
\includegraphics[scale=0.7]{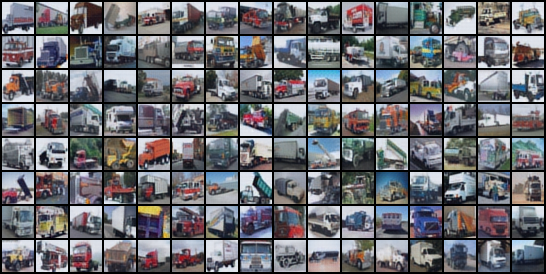}
\label{fig:cifar_5}
\end{figure}

\subsection{ImageNet-50}
\begin{figure}[H]
\centering
\includegraphics[scale=0.7]{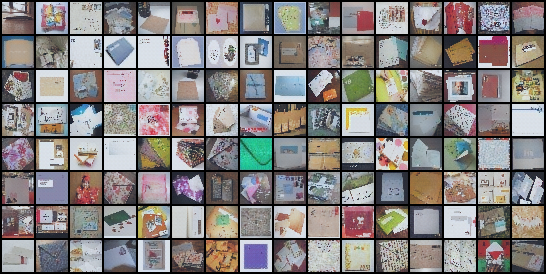}
\label{fig:imagenet_0}
\end{figure}

\begin{figure}[H]
\centering
\includegraphics[scale=0.7]{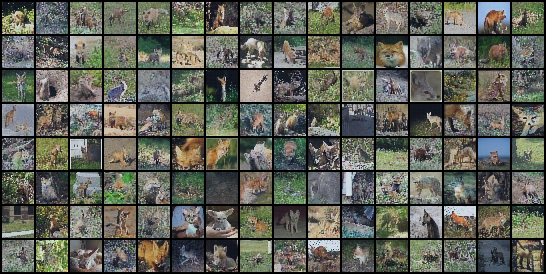}
\label{fig:imagenet_1}
\end{figure}

\begin{figure}[H]
\centering
\includegraphics[scale=0.7]{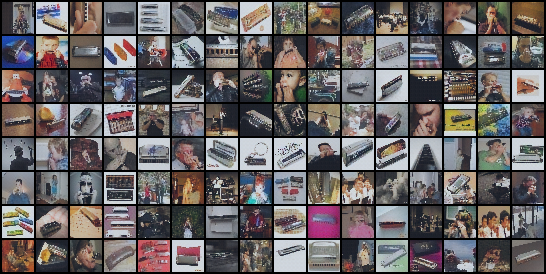}
\label{fig:imagenet_2}
\end{figure}

\begin{figure}[H]
\centering
\includegraphics[scale=0.7]{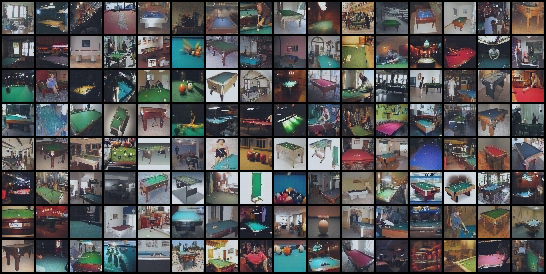}
\label{fig:imagenet_3}
\end{figure}

\begin{figure}[H]
\centering
\includegraphics[scale=0.7]{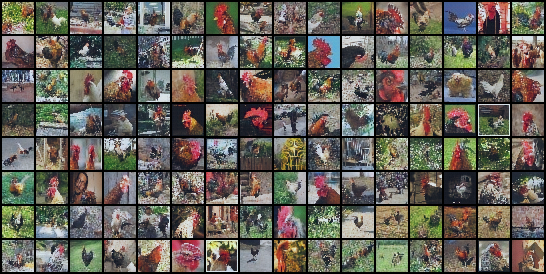}
\label{fig:imagenet_4}
\end{figure}

\begin{figure}[H]
\centering
\includegraphics[scale=0.7]{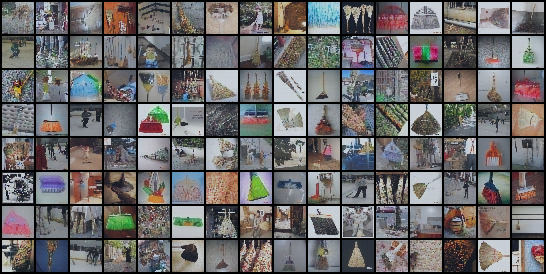}
\label{fig:imagenet_5}
\end{figure}
